# Supplementary material for: Sensitivity potential to a light flavor-changing scalar boson with DUNE and NA64$\mu$
Source: arXiv:2306.07405 source file (2023-06-12)
Supplement: Supplementary file 1 [file appendix.tex]

Both in cross-section and decay width calculations phase-space factors show up. The general form of these integrals are 
\begin{equation}
    \sigma \propto \int |\mathcal{M}|^2 \cdot R_{n} 
\end{equation}
where $\mathcal{M}$ is the quantum-field theoretical amplitude, containing the interactions between particles in a process, while $R_{n}$ is the N-body final-state phase-space factor. Because we are mostly interested in average quantities we integrate or sum over all possible final-state kinematics. The general phase-space factor for a process going from an initial state $P_i = p_1 + p_2$ to final state $P_f = p_1' + p_2' + \dots + p_n'$ is expressed formally as follows 

\begin{align*}
R_{n}& = \int d^4p_1' \int d^4p_2' \dots \int d^4p_n' \\
& \times \delta^4(p_1' + p_2' + \dots + p_n' - p_1 - p_2)\\
&\times \prod_{i=1}^{n} \delta(p_i'^2 - m_i^2)
\label{Eq:Rndef}
\end{align*}

Here the first $\delta$-function ensures that during the integral only those initial and final states are included for which the energy and momentum are conserved. The second product of $n$ $\delta$-functions formally express that the final-state particles have a finite mass. Therefore, the phase-space factor restricts the contributions to the cross-section or decay width integrals to those that are \textit{kinematically} allowed. It can be thought of as a weighting factor that assigns a non-zero weight to the kinematically allowed final states and a zero weight to the kinematically forbidden final states. But even when the weight is non-zero, the probability of partitioning the final-state to random configurations is not uniform.

Two widely-cited resources in the literature \cite{FJames, Hagedorn} derive the general formula for N-body phase-space factors in the rest frame ($P = (M,\vec{0})$) of decaying particle with mass $M$. This can be generalized to collisions with initial four-momenta $P = p_1 + p_2$ and boosting the ``particle'' $P$ into its rest frame. The main idea is to reduce the N-body phase-space calculation recursively to a N-1-body phase-space problem. For example, a 3-body process $M\rightarrow m_1 + m_2 + m_3$ is reduced to two 2-body processes: $M\rightarrow M_{1,2} + m_3$ and $M_{1,2} \rightarrow m_1 + m_2$, where $M_{1,2}$ is the two-particle system made up of particles $m_{1}$ and $m_{2}$ with four-momenta $p_1$ and $p_2$. Kinematically, $M_{1,2}$ is limited to the following range
\begin{equation}
    m_1 + m_2 \leq M_{1,2} \leq M - m_{3}
    \label{Eq:limits}
\end{equation}

which intuitively makes sense: the minimal energy $M_{1,2}$ could have is the sum of the rest masses of its constituents, and the maximal available energy is the mass of the parent particle $M$ minus the rest mass of the other particle (i.e. the other particle is just created at threshold).
That allows us to do following: generate initial and final states for an event basically in any way (as long as energy and momentum are conserved), but then weight them with the following phase-space factor to get the kinematically correct distribution:
\begin{equation}
    w_{n} = R_{n-l+1}(P;M, m_{l+1}, \dots, m_{n})\times R_{l}(P_{l}; m_{1},\dots, m_{l})
\label{Eq:weight}
\end{equation}
where $R_{n-l+1}(P;M, m_{l+1}, \dots, m_{n})$ is the phase-space factor when there are $n-1$ particles, $m_{l+1}, \dots, m_{n}$, plus one extra particle with mass $M^2=P_{l}^2$. In this situation, the extra particle $P_{l}$ represents the remaining system of $m_{1}, \dots, m_{l}$ particles as a single object. And $R_{l}(P_{l}; m_{1},\dots, m_{l})$ is the phase-space factor describing that extra particle, $P_{l}$. The weight $w_n$ is to be normalized by the maximum weight, which will be given below.

%The 1-body phase-space factor for a particle at rest ($\vec{p} = \vec{0}$) is

%\begin{equation}
%    R_{1}(E;m) = \int \frac{d^3 p}{2\sqrt{\vec{p}^{2} + m^{2}}} \delta(E-\sqrt{\vec{p}^2 + m^2})\delta^3(\vec{p}) = \frac{\delta(E-m)}{2m}
%\end{equation}

The 2-body phase-space factor for a process $M\rightarrow m_{1} + m_{2}$ in the rest frame of a particle $M$ ($P = (M, \vec{0})$; $M^2 = P^2 = (p_{1} + p_{2})^2$) is as follows

\begin{equation}\label{Eq:2bodyPS}
   R_{2}(M; m_1, m_2) = \frac{\pi}{2M^2} \sqrt{[M^2 - (m_{1} + m_{2})^2][M^2 - (m_{1} - m_{2})^2]} = \frac{\pi}{M}p(M; m_1, m_2). 
\end{equation}

where it is noted that $p$ is the magnitude of the three-momentum of the daughter particles in the CM frame
\begin{equation*}
    p^2(M; m_1, m_2) = \frac{[M^2 - (m_{1} + m_{2})^2][M^2 - (m_{1} - m_{2})^2]}{4M^2}
\end{equation*}

From the general equation Eq.~\ref{Eq:weight} above we can express the 3-body phase-space factor for the decay $M \rightarrow m_1 + m_2 + m_3$ as a product of two factors: (1) a phase-space factor describing the decay $M \rightarrow M_{1,2} + m_3$ with $M_{1,2}$ representing a composite ``particle'' $\{m_1,m_2\}$, and (2) a phase-space factor describing the ``decay'' of the composite ``particle'' $M_{1,2}\rightarrow m_{1} + m_{2}$, with $M_{1,2} = \sqrt{p_{1}^2 + p_{2}^2}$,

\begin{equation}
    R_{3}(M; m_1, m_2, m_3) = \frac{\pi^2}{M M_{1,2}}p(M; M_{1,2}, m_3)\times p(M_{1,2}; m_1, m_2) 
\end{equation}

The \textit{largest weight}, $w^{\mathrm{max}}_{n}$ will be obtained when the function $p$ gets its maximum value \footnote{Note that the general $\pi/M$ factors may be dropped because they cancel in the overall normalization for the maximum weight.}. For the 3-body decay, this occurs roughly when $M$ is maximal and $M_{1,2}$ is minimal (the first $p$ factor), and $M_{1,2}$ is maximal and $m_1$ is minimal (second $p$ factor). We saw that for the intermediate composite particle $M_{1,2}$, in the 3-body decay the upper limit is given in Eq.~\ref{Eq:limits}. Therefore, we can identify that the largest weight occurs for $R_3$ with 
\begin{align*}
    p^{\mathrm{max}}(M; M_{1,2}, m_3)& = p(M; m_1+m_2, m_3)\\ 
    p^{\mathrm{max}}(M_{1,2}; m_1, m_2) & = p(M-m_3, m_1, m_2)
\end{align*}
This generalizes for larger number of final states, $N$, as well. But for this tutorial N=3 is enough. So for a 3-body decay the normalized event weight becomes 
\begin{equation}
    \frac{w_3}{w_3^{\mathrm{max}}} = \frac{R_{3}(M; m_1, m_2, m_3)}{R_{3}^{\mathrm{max}}(M; m_1, m_2, m_3)} = \frac{p(M; M_{1,2}, m_3)\times p(M_{1,2}; m_1, m_2)}{p(M; m_1+m_2, m_3)\times p(M-m_3, m_1, m_2)} 
\end{equation}
The normalization factor is a constant (it contains only rest masses), but the numerator is not: the 3-body phase-space weights will have a distribution because $M_{1,2} = \sqrt{p_1^2 + p_2^2}$ and the components in the four-vectors $p_1$ and $p_2$ depend on the random final state. However, for a 2-body final state the phase-space factor is constant, see Eq.~\ref{Eq:2bodyPS}.
